# Supplementary material for: Causal Strategic Linear Regression
Source: arXiv:2002.10066 source file (2022-08-25)
Supplement: Supplementary file 2 [file supplement.tex]

\documentclass{article}

% Recommended, but optional, packages for figures and better typesetting:
\usepackage{microtype}
\usepackage{graphicx}
\usepackage{subfigure}
\usepackage{booktabs} % for professional tables
\usepackage{algorithm, algorithmic}
\usepackage{amsmath,amsthm,amssymb}
\usepackage{thmtools}
\usepackage{xcolor}
\usepackage{verbatim}



% hyperref makes hyperlinks in the resulting PDF.
% If your build breaks (sometimes temporarily if a hyperlink spans a page)
% please comment out the following usepackage line and replace
% \usepackage{icml2020} with \usepackage[nohyperref]{icml2020} above.
\usepackage{hyperref}

% Attempt to make hyperref and algorithmic work together better:
\newcommand{\theHalgorithm}{\arabic{algorithm}}

% Use the following line for the initial blind version submitted for review:
\usepackage{icml2020/icml2020}

% If accepted, instead use the following line for the camera-ready submission:
% \usepackage[accepted]{icml2020/icml2020}

% The \icmltitle you define below is probably too long as a header.
% Therefore, a short form for the running title is supplied here:
\declaretheorem{theorem}
\declaretheorem{corollary}
\declaretheorem{lemma}
\declaretheorem{observation}
\declaretheorem{proposition}
\declaretheorem{definition}
\declaretheorem{claim}
\declaretheorem{fact}
\declaretheorem{question}
\declaretheorem[style=definition]{objective}

\newcommand{\N}{\mathbb{N}}
\newcommand{\Z}{\mathbb{Z}}
\newcommand{\R}{\mathbb{R}}
\newcommand{\w}{\omega}
\newcommand{\agentdist}{P} 
\newcommand{\agentspace}{\mathcal{X}}
\newcommand{\gamedagentdist}[1]{P_{#1}}
\newcommand{\acspace}{A}
\newcommand{\approxclass}{\mathcal{H}} % Approximator class
\newcommand{\E}[2][\space]{\mathbb{E}_{#1} \left [ #2 \right ]}
\newcommand{\datasetatround}[1]{D^{(#1)}}
\newcommand{\bern}[1]{\text{Bern}(#1)}
\newcommand{\proj}{\text{proj}}

\newcommand{\yonote}[1]{\textcolor{magenta}{#1}}
\newcommand{\bennote}[1]{\textcolor{blue}{#1}}
\newcommand{\briannote}[1]{\textcolor{green}{#1}}

\DeclareMathOperator*{\argmax}{arg\,max}
\DeclareMathOperator*{\argmin}{arg\,min}


% hyperref makes hyperlinks in the resulting PDF.
% If your build breaks (sometimes temporarily if a hyperlink spans a page)
% please comment out the following usepackage line and replace
% \usepackage{icml2020} with \usepackage[nohyperref]{icml2020} above.
\usepackage{hyperref}

% Attempt to make hyperref and algorithmic work together better:

% Use the following line for the initial blind version submitted for review:
\usepackage{icml2020/icml2020}

% If accepted, instead use the following line for the camera-ready submission:
%\usepackage[accepted]{icml2020}

% The \icmltitle you define below is probably too long as a header.
% Therefore, a short form for the running title is supplied here:
\icmltitlerunning{Supplement to ``Learning From Strategic Agents''}

\begin{document}

\onecolumn%[
\icmltitle{Supplementary Material to 
``Learning From Strategic Agents: Accuracy, Improvement, and Causality''
}
         

% It is OKAY to include author information, even for blind
% submissions: the style file will automatically remove it for you
% unless you've provided the [accepted] option to the icml2020
% package.

% List of affiliations: The first argument should be a (short)
% identifier you will use later to specify author affiliations
% Academic affiliations should list Department, University, City, Region, Country
% Industry affiliations should list Company, City, Region, Country

% You can specify symbols, otherwise they are numbered in order.
% Ideally, you should not use this facility. Affiliations will be numbered
% in order of appearance and this is the preferred way.

\begin{icmlauthorlist}
\icmlauthor{Yonadav Shavit}{harvard}
\icmlauthor{Benjamin L. Edelman}{harvard}
\icmlauthor{Brian Axelrod}{stanford}
\end{icmlauthorlist}

\icmlaffiliation{harvard}{John A. Paulson School of Engineering and Applied SCiences, Harvard University, Cambridge, MA, USA}
\icmlaffiliation{stanford}{Department of Computer Science, Stanford University, Stanford, California, USA}

\icmlcorrespondingauthor{Yonadav Shavit}{yonadav@g.harvard.edu}
%]
% this must go after the closing bracket ] following \twocolumn[ ...

% This command actually creates the footnote in the first column
% listing the affiliations and the copyright notice.
% The command takes one argument, which is text to display at the start of the footnote.
% The \icmlEqualContribution command is standard text for equal contribution.
% Remove it (just {}) if you do not need this facility.

\printAffiliationsAndNotice{}  % leave blank if no need to mention equal contribution
% \printAffiliationsAndNotice{\icmlEqualContribution} % otherwise use the standard text.
\appendix
\input{appA_causal}
% \section{Causal Precision}
% In this section we describe how we recover $\hat\omega_{opt}$ in $\L_2$ when there exists an $\omega$ such that $\Sigma + G \omega$ is full rank. Before we proceed we make a couple of observations. When there is no way to make the above matrix full rank, we cannot hope to recover the optimal $\hat\omega_{opt}$. If there is no natural variation in e.g. the last two features, and furthermore no agent can act along those features, it is not possible to disentangle their potential effects on the outcome. This also suggests that the causal precision is a more substantive demand for the decision maker than the standard linear regression setting. To discover this additional information, the decision maker can incentivize the agents to take actions that help the decision-maker recover the true outcome-governing parameters.

% This motivates the algorithm we present in this section. It operates in two stages. First, it recovers the information necessary in order to to identify the decision rule which will provide the most informative agent samples after those agents have gamed. Second, it collects data while incentivizing this action. Finally, it computes an estimate of $\hat\omega_{opt}$ using the collected data. We present the complete procedure in Algorithm \ref{alg:causal}. 

% \begin{algorithm*}
%   \caption{Recovering the Causal Model} 
%   \label{alg:causal}
% %  \textbf{Input}: $X_n = (x_1, x_2, \dots, x_n)$, where $x_i \leftarrow N(\mu, \Sigma_{d \times d})$.\\
% %   \textbf{Output}: $Z_m = (x_1', x_2', \dots, x_m')$, such that $D_{TV}(D^m, Z_m) \leq \frac{1}{3}$, where $D$ is $N(\mu, \Sigma_{d \times d})$
%   \begin{algorithmic}[1]
%   \STATE Let $k_1 = \lambda_{max}(G^TG)$ and $k_2 = || \Sigma ||^2$
%   \STATE Choose an $\epsilon > 0$
%   \STATE Let $n_1 = O(\max (\frac{d k_1}{\kappa_{min}}, \frac{d^2 k_2}{\kappa_{min}}) )$
%   \STATE Collect samples $x_1,\ldots,x_{n_1}$
%   \STATE Let $\hat \mu = \frac{1}{n_1}\sum x_i$
%   \STATE Let $\hat \Sigma = \frac{1}{n_1}\sum x_ix_i^T$
%   \STATE Let $n_2 = O( \max({d^2 ||\hat\mu||^2 \mathrm{tr}(\Sigma), d^3 ||G||^2 \mathrm{tr}(\Sigma)  }))$
%   \FOR{ $i = 1...d$}
%   \STATE $\omega = e_i$
%   \STATE Sample $x_1, \ldots, x^i_{n_2}$ and subtract $\hat \mu$ from each one. 
%   \STATE Let $\hat G_i = \frac{1}{n_2} \sum\limits_{j = 1}^{n_2} x_j$ 
%   \ENDFOR
%   \STATE Let $\hat\omega_{opt} = \argmin\limits_{\omega} \hat \Sigma + 2 \mu \omega^T \hat G^T +  \hat G \omega \omega^T \hat G ^T $
%   \STATE Let $n_3 = O(\frac{d}{\epsilon \kappa_{min}})$ 
%   \STATE Sample $x_1,\ldots, x_{n_3}$ with $\omega = \hat\omega_{opt}$. 
%   \STATE Return the output of OLS on $x_1,\ldots, x_{n_3}$
%   \end{algorithmic}
% \end{algorithm*}

% The procedure in Algorithm \ref{alg:causal} can be summarized as follows: 
% \begin{enumerate}
%     \item Estimate the first and second moments of the distribution of agents' features.
%     \item Estimate the action matrix $G$.
%     \item Compute the most informative choice of $\omega$.
%     \item Collect samples under the most informative $\omega$ and then return the output of OLS.
% \end{enumerate}

% Before we proceed to the proof of correctness of Algorithm \ref{alg:causal}, let us build some intuition for why this procedure of choosing a single $\omega$ and collecting samples under said $\omega$ makes sense. As we show later, the convergence of OLS for linear regression can be controlled by the minimum eigenvalue of the second moment matrix of the samples. Our algorithm finds the value of $\omega$ that, after agents game, maximizes this minimum eigenvalue in expectation. It turns out the minimum eigenvalue of the expected second moment matrix of post-gaming samples is convex with respect to the choice of $\omega$. The convexity of the objective suggests that a priori, when choosing $\omega$s to obtain informative samples, the optimal strategy is choose a single specific $\omega$. 

% The main difficulty in the rest of the algorithm is achieving the necessary precision in the estimation to be able to set up the above optimization problem to identify such an $\omega$. 

% \begin{theorem}\label{thm:causal}
% When $V = I$, the output of Algorithm \ref{alg:causal} run with parameter $\epsilon$ satisfies $|| \omega - \omega^*|| \le \epsilon$ with probability greater than $\frac 2 3$.
% \end{theorem}

% The proof of Theorem \ref{thm:causal} relies on several lemmas. First we bound the $L_2$ error of OLS as a function of the empirical second moment matrix in Lemma \ref{lem:olsell2}. Note that the usual bound for the convergence of OLS is distribution dependent. That is, the expected error is small. 

% \begin{lemma}\label{lem:olsell2}
% Assume $V = I$. Consider samples $x_1,\ldots, x_n$ and $y_i = {\hat\omega_{opt}}^T x_i + \eta_i$. Let $\omega$ be the output of OLS $(x_i, y_i)$. Then 
% $$ \mathbb E_{\eta}\left [ || \omega - \hat\omega_{opt}|| ^2 \right] \le \frac{d}{n \kappa_{min}}$$
% \end{lemma}
% The above proof is elementary and a slight modification of the standard textbook proof (see for example, \cite{liangstat}).

% The proof also requires that the optimization to choose the optimal $\omega$ is convex. 
% \begin{lemma}\label{lem:convex}
% The minimum eigenvalue of the following matrix is convex with respect to $\omega$ for any values of $x,G$. 
% $$ \sum\limits_i (x_i + \hat G \omega)(x_i + \hat G \omega)^T$$ 

% Furthermore, when the following conditions are true, then the minimum eigenvalue of the above is within a constant factor of the optimal value. 

% $\mathbb E[(x + G \omega)(x + \hat G \omega)^T ]$. 

% \begin{itemize}
%     \item $|| \hat \Sigma - \Sigma ||^2 \le \epsilon$
%     \item $|| \mu - \hat \mu || ^2 \le \frac{\lambda_{max}(G^T G) \epsilon }{d}$
%     \item $ ||\hat G - G||^2 \le \frac{\epsilon}{d || \mu ||^2}$
%     \item $ || \hat G - G ||^2 \le \frac{\epsilon}{d^2 || G ||^2}$
% \end{itemize}

% Finally, the above holds true even for an $\omega$ with distance at most $O(\frac{1}{poly(d)})$ from the optimum.
% \end{lemma}

% Finally, we use a minor lemma for recover of a random vector via the empirical mean estimator. Note that we treat the matrix $G$ as a vector. 
% \begin{lemma}\label{lem:grec}
% Assume $V = I$. Let $g_1^i,\ldots, g_n^i$ be drawn from the distribution $G_i + \xi$ and $\hat G$ be the empirical mean estimator computed from said $g_j^i$'s. 
% Let $\Sigma$ be the expected second moment matrix of the $\xi$s. 
% Then $$ \mathbb E_\xi ||G - \hat G ||^2 \le \frac{d^2 \mathrm{tr}(\Sigma)}{n}$$
% \end{lemma}

% We proceed with the proof of Theorem \ref{thm:causal} below. 

% \begin{proof}
% The first step of the algorithm is for recovering an estimate of $\Sigma$ and $\mu$.
% Note that $n_1$ samples suffice to recover $\hat \Sigma$ and $\hat \mu$ such that:
% \begin{itemize}
%     \item $|| \hat \Sigma - \Sigma ||^2 \le \epsilon$
%     \item $|| \mu - \hat \mu || ^2 \le \frac{\lambda_{max}(G^T G) \epsilon }{d}$
% \end{itemize}

% The for loop recovers an estimate of $G$. Via Lemma \ref{lem:grec}, the samples suffice to ensure that the following two conditions hold: 
% \begin{itemize}
%     \item $ ||\hat G - G||^2 \le \frac{\epsilon}{d || \mu ||^2}$
%     \item $ || \hat G - G ||^2 \le \frac{\epsilon}{d^2 || G ||^2}$
% \end{itemize}

% Then the algorithm computes an estimate of the optimal $\omega$. Via Lemma \ref{lem:convex}, we have that the optimum guarantees the minimum eigenvalue of an approximate solution will be within a constant factor of the optimum. 

% This $\omega$ guarantees that $n_3$ samples suffice to ensure the recover of $\omega^*$ within squared $\L_2$ distance of $O(\epsilon)$ in expectation. 

% Finally the expectations can be used with a Markov inequality to ensure the algorithm succeeds with (arbitrarily high) constant probability. 
% \end{proof}

% Now we prove the lemmas. 
% We begin with Lemma \ref{lem:olsell2}. This proof is a slight modification of the textbook proof for the convergence of OLS. 

% \begin{proof}
% In this section we derive a bound on the convergence of the least squares estimator when a fixed design matrix $X$ is used. Note this is exactly the case we encounter, since the choice of $\omega$ lets us affect the entries of the design matrix. This is a standard, textbook result and not a main contribution of the paper. 

% In order to state the result more formally we have to introduce some notation. The goal of the procedure is to recover $\hat\omega_{opt}$, when given tuples $(x_i, \hat\omega_{opt} x_i + \eta)$ where $\eta$ is 1-subgaussian. We aim to characterize $||\omega - \hat\omega_{opt} || $ where $\omega$ is obtained from ordinary least squares. Let $X$ be the vector with the $x_i$'s in its columns. Let $\kappa_{min}$ be the minimum eigenvalue of $\frac 1 n X^TX$ (the second moment matrix).  

% Below all expectations are taken \emph{only} over the random noise. We assume the second moment matrix is full rank.

% \begin{align*}
%     \mathbb E[|| \omega - \hat\omega_{opt}|| ^2] &\le \mathbb E[ \frac{1}{n\kappa_{min}}  (\omega - \hat\omega_{opt}) X^T X (\omega - \hat\omega_{opt})]\\
%     & = \mathbb E[\frac{1}{n\kappa_{min}} || X (\omega - \hat\omega_{opt})|| ^2] \\
%     &= \frac{1}{n\kappa_{min}} \mathbb E[|| X(X^TX)^{-1}X^T (X \hat\omega_{opt} + \eta) - X\hat\omega_{opt}|| ^2]\\
%     &= \frac{1}{n\kappa_{min}} \mathbb E[|| X(X^TX)^{-1}X^T \eta|| ^2]\\
%     &\le \frac{d}{n \kappa_{min}}
% \end{align*}

% This motivates our procedure to learn the causal model. We do so in a fashion that attempts to maximize $\kappa_{min}$. Note that it is the mininum eigenvalue that determines the convergence rate. This is due to the fact that little variation along a dimension makes it hard to dissentangle the features' effect on the outcome via $\hat\omega_{opt}$ from the constant-variance noise $\eta$.  
% \end{proof}

% Lemma \ref{lem:convex} is somewhat more involved. It is proven in three parts. The first is that the optimization problem is convex. The second is that approximate recovery of $S, \mu,$ and  $G$ suffice for approximately minimizing the original expression. The third is that an approximate solution suffices. 

% \begin{proof}
% In this section we describe how to choose the value of $\omega$ that maximizes the value of $\kappa_{min}$ for the samples we obtain. 

% To do so, we examine the expectation of the second moment matrix and make several observations. Let $\Sigma$ denote the expected second moment matrix of $x$ (i.e. $\mathbb E[xx^T]$. We have: 
% $$ \mathbb E[(x + G \omega) (x + G \omega)^T] = \Sigma + 2 \mu \omega^T G^T + G \omega \omega^T G^T$$
% \begin{enumerate}
%     \item The minimum eigenvalue of the above expression is concave with respect to $\omega$. This follows due to the following: $x + G \omega$ is a linear operator, the minimum eigenvalue of a Gramian matrix $X^T X$ is concave with respect to $X$ and the expectation of a concave function is concave \cite{boyd2004convex}. 
%     \item Since the agent attempts to maximize their motion in the $\omega$ direction, we want to ensure that we move them toward toward the direction that maximizes the minimum eigenvalue of $\mathbb E[ (x + G \omega) (x + G \omega)^T]$. 
% \end{enumerate}

% However, we do not operate with exact knowledge of $G$, etc. It turns out that even approximately solving this optimization problem with estimates for $G, \Sigma, \mu$ suffices for our purposes, as long as the $\omega$ we obtain from our optimization (using the estimates) results in a high value for the minimum eigenvalue of $\mathbb E[(x + G \omega) ( x + G \omega)^T] $. Let $\hat \omega$ be the maximizing argument for the estimated optimization problem and let $\omega$ be the maximizing argument for the original optimization problem. Let $Q$ be the true maximized second moment matrix including gaming, and $\hat Q$ be the maximizing second moment matrix with gaming resulting from replacing the true $\Sigma, \mu, G$ with the estimates. In formal terms, we need to show the minimum eigenvalue of the following is large: $ \mathbb E [(x + G \hat \omega) (x + G \hat \omega)^T] $. 
% We note that when $y^T \hat Q y$ is within $\epsilon$ of $y^T Q y$ for all $y$ in the unit ball, the minimum eigenvalues may differ by at most $\epsilon$. 
% \begin{align*}
%     || y^T \hat Q y - y ^T Q y||^2 &= || y^T (\hat Q - Q) y||^2\\
%     &\le \lambda_{max}^2 (\hat Q - Q)(y) || y ||^2\\
%     & \le || \hat Q - Q||^2 
% \end{align*}

% And now we bound the norm of $|| \hat \Sigma - \Sigma ||^2$ assuming the following:
% \begin{enumerate}
%     \item $|| \hat \Sigma - \Sigma||^2 \le \epsilon $
%     \item $|| \mu - \hat \mu ||^2 \le \frac{\lambda_{max}(G^T G) \epsilon}{d}$
%     \item $|| \hat G - G ||^2 \le \frac \epsilon {d ||\mu||^2}$
%     \item $|| \hat G - G ||^2 \le \frac{\epsilon} {d^2 || G ||^2}$
% \end{enumerate}

% We work out the bound below. 
% \begin{align*}
%     || \hat Q - Q ||^2 &= || \Sigma + 2 \mu {\hat\omega_{opt}}^T G^T + G \hat\omega_{opt} {\hat\omega_{opt}}^T G^T - (\hat \Sigma + 2 \hat \mu \omega^T \hat G^T + \hat G  \hat\omega_{opt} {\omega_{opt}}^T \hat G^T)||^2\\
%     &\le || \Sigma - \hat \Sigma|| ^2 + 2||  \mu {\hat\omega_{opt}}^T G^T -  \hat \mu {\hat\omega_{opt}}^T \hat G^T|| ^2 + || \ldots|| ^2\\
%     & \le \epsilon + 2||  \mu {\hat\omega_{opt}}^T G^T  + {\hat \mu \hat\omega_{opt}}^TG^T- {\hat \mu \hat\omega_{opt}}^TG^T-  \hat \mu {\hat\omega_{opt}}^T \hat G^T|| ^2 + || \ldots|| ^2\\
%     &\le \epsilon + d|| \mu - \hat \mu||^2 ||  {\hat\omega_{opt}}^T G ||^2 + || \hat G - G||^2 || \hat \mu \omega^T||^2 + \ldots\\
%     &\le \epsilon + \epsilon + || \hat G - G||^2 || \hat \mu \omega^T  +\mu  \omega^T - \mu \omega^T ||^2 + \ldots\\
%     &\le \epsilon + \epsilon + || \hat G - G||^2 (|| \hat \mu - \mu||^2 + || \mu {\hat\omega_{opt}}^T||) + \ldots\\
%     & \le \epsilon + \epsilon + || \hat G - G||^2 d || \mu||^2 + \ldots\\
%     & \le 3 \epsilon + || \hat G  \hat\omega_{opt} {\hat\omega_{opt}}^T \hat G^T -  G  \hat\omega_{opt} {\hat\omega_{opt}}^T G^T ||^2\\
%     &\le 3 \epsilon + || \hat G  \hat\omega_{opt} {\hat\omega_{opt}}^T \hat G^T - \hat G \hat\omega_{opt} {\hat\omega_{opt}}^T G + \hat G \hat\omega_{opt} {\hat\omega_{opt}}^T G -  G  \hat\omega_{opt} {\hat\omega_{opt}}^T G^T ||^2\\
%     &\le 3 \epsilon + || (\hat G - G)  \hat\omega_{opt} {\hat\omega_{opt}}^T \hat G^T ||^2 + || (\hat G - G)  \hat\omega_{opt} {\hat\omega_{opt}}^T G^T ||^2\\
%     & \le 3 \epsilon + || (\hat G - G)  \hat\omega_{opt} {\hat\omega_{opt}}^T \hat G^T - (\hat G - G)  \hat\omega_{opt} {\hat\omega_{opt}}^T G^T + (\hat G - G)  \hat\omega_{opt} \hat\omega_{opt}^T  G^T ||^2 + d^2|| \hat G - G||^2 ||G ||^2\\
%     & \le 4 \epsilon  + ||(\hat G - G)  \hat\omega_{opt} {\hat\omega_{opt}}^T  (\hat G - G) ||^2 + || (\hat G - G)  \hat\omega_{opt} {\hat\omega_{opt}}^T G^T ||^2\\
%     & \le 5 \epsilon + d^2 || \hat G - G||^4 \\
%     & \le 6 \epsilon 
% \end{align*}

% This means if we find an $\epsilon-$approximate solution to the system with the estimated values, we obtain a $\kappa_{min}$ within $6\epsilon$ of the optimal. 
% \end{proof}

% Finally the proof of Lemma \ref{lem:grec}. 
% \begin{proof}
% Recall that when the decision-maker fixes $\omega$, it receives samples of the form $x + G \omega$. We note this can be used to recover the matrix $G$. In particular, we show how $d$ rounds, each with $O(\frac{d \mathrm{tr}(\Sigma)}{\epsilon})$ samples, suffices to recover the matrix to squared frobenius norm $\epsilon$. 
% Recall the procedure we propose simply chooses $\omega = e_1,...e_d$, one-hot coordinate vectors in each round. 
% We first bound the error in $\hat G$. coordinate-wise:  $\mathbb E[||\hat G_{i,j} - G_{i,j}||^2] \le \frac{\mathbb E[x_i^2]}{n}$. A union bound across coordinates shows that $O(\frac{d^2 \mathrm{tr}(\Sigma)}{\epsilon})$ samples suffice to recover $G$ within squared Frobenius norm $\epsilon$.
% \end{proof}

 

  % TODO check that the minimum eigenvalue of the empirical second moment matrix is within a constant factor of the proper one. 
%TODO describe the complete algorithm. 

% TODO work out the sensitivity

\bibliography{bibliography}
\bibliographystyle{icml2020/icml2020}


\end{document}


% This document was modified from the file originally made available by
% Pat Langley and Andrea Danyluk for ICML-2K. This version was created
% by Iain Murray in 2018, and modified by Alexandre Bouchard in
% 2019 and 2020. Previous contributors include Dan Roy, Lise Getoor and Tobias
% Scheffer, which was slightly modified from the 2010 version by
% Thorsten Joachims & Johannes Fuernkranz, slightly modified from the
% 2009 version by Kiri Wagstaff and Sam Roweis's 2008 version, which is
% slightly modified from Prasad Tadepalli's 2007 version which is a
% lightly changed version of the previous year's version by Andrew
% Moore, which was in turn edited from those of Kristian Kersting and
% Codrina Lauth. Alex Smola contributed to the algorithmic style files.
