# Supplementary material for: Causal Strategic Linear Regression
Source: arXiv:2002.10066 source file (2022-08-25)
Supplement: Supplementary file 3 [file suppbak.tex]

\subsection{OLS Second Moment Dependance}
In this section we derive a bound on the convergence of the least squares estimator when a fixed design matrix is used. Note this is exactly the case we encounter, since the choice of $\omega$ lets us affect the entries of the design matrix. This is a standard, textbook result and not a main contribution of the paper. 

In order to state the result more formally we have to introduce some notation. The goal of the procedure is to recover $\omega^\star$, when given tuples $(x_i, \omega^\star x_i + \epsilon_i)$ where $\epsilon$ is 1-subgaussian. We aim to characterize $||\omega - \omega^\star || $ where $\omega$ is obtained from ordinary least squares. Let $X$ be the vector with $x_i$'s in it's columns. Let $\kappa_{min}$ be the minimum eigenvalue of $\frac 1 n X^TX$ (the second moment matrix).  

Below all expectations are taken \emph{only} over the random noise. We assume the second moment matrix is full rank.


\begin{align*}
    \mathbb E[|| \omega - \omega^\star|| ^2] &\le \mathbb E[ \frac{1}{n\kappa_{min}}  (\omega - \omega^\star) X^T X (\omega - \omega^\star)]\\
    & = \mathbb E[\frac{1}{n\kappa_{min}} || X (\omega - \omega^\star)|| ^2] \\
    &= \frac{1}{n\kappa_{min}} \mathbb E[|| X(X^TX)^{-1}X^T (X \omega^\star + \epsilon) - X\omega^\star|| ^2]\\
    &= \frac{1}{n\kappa_{min}} \mathbb E[|| X(X^TX)^{-1}X^T \epsilon|| ^2]\\
    &= \frac{d}{n \kappa_{min}}
\end{align*}

This motivates our procedure to learn the causal classifier. We do so in a fashion that attempts to maximize $\kappa_{min}$. Note that it is the mininum eigenvalue that determines the convergence rate. This is due to the fact that little variation along a dimension makes it hard to dissentangle signal from $\omega^\star$ from the constant variance noise. 
 % TODO cite the notes https://web.stanford.edu/class/cs229t/notes.pdf

\subsection{Recovering the action matrix via OLS}
In this section we show how one can recover the action matrix. Recall that when the decision-maker fixes $\omega$, it receives samples of the form $x + G \omega$. We note this can be used to recover the matrix $G$. In particular, we show how $d$ rounds, each with $O(\frac{d \mathrm{tr}(\Sigma)}{\epsilon})$ samples, suffices to recover the matrix to squared frobenius norm $\epsilon$. 

The procedure we propose simply chooses $\omega = (e_1,...e_d)$, one-hot coordinate vector in each round. We when compute an OLS estimate of each row of the matrix. We note this identical to a larger OLS which recovers the matrix in one go. We let $\hat G$ denote the OLS solution and $G_i$ denote the $i$th row the matrix $G$. We continue to use $X$ to denote the design matrix, noting that in this case, $x_{i}$ represents the random variable corresponding to vector of the $i$th coordinates of the samples and not a part of the design matrix. This results in a second moment matrix of $\frac 1 d I$. Though we were not able find a reference, we believe this is a standard procedure and not a main contribution of the paper. 

\begin{align*}
    \mathbb E[|| G - \hat G||^2] &= \sum\limits_i \mathbb E[ || G_i - \hat G_i||^2 ] \yonote{\text{how does second line follow?}}\\
    &= \frac{1}{n}\sum\limits_i \mathbb E[ || X(\hat G_i -  G_i)||^2 ]\\
    &= \frac{1}{n}\sum\limits_i \mathbb E[ || X(X^T X)^{-1} X^T(X  G_i + x_i) + X G_i ||^2 ]\\
    &= \frac{1}{n}\sum\limits_i \mathbb E[ || X(X^T X)^{-1} X^T x_i ||^2 ]\\
    &= \frac{1}{n}\sum\limits_i\mathbb E[ ||  (x_i) ||^2d ]\\
    &= \frac{d^2 \mathrm{tr}(S)}{n}
\end{align*}

\subsection{Choosing the Optimal $\omega$ for recovery of the causal estimator} 
Recall that the first result depends on the value of $\kappa_{min}$, the minimum eigenvalue of the design matrix. In this section we describe how to choose the value of $\omega$ that maximizes the value of $\kappa_{min}$ for the samples we obtain. 

To do so, we examine the expectation of the second moment matrix and make several observations. Let $S$ denote the expected second moment matrix of $x$ (i.e. $\mathbb E[xx^T]$. 
$$ \mathbb E[(x + G \omega) (x + G \omega)^T] = S + 2 \mu \omega^T G^T + G \omega \omega^T G^T$$
\begin{enumerate}
    \item The minimum value is concave with respect to $\omega$. This follows due to the following: $x + G \omega$ is a linear operator, the minimum eigenvalue of a Gramian matrix $X^T X$ is concave with respect to $X$ and the expectation of a concave function is concave \cite{boyd2004convex}. 
    \item Since the agent attempts to maximize the value in the $\omega$ direction, the value for which the solution to the maximization of the above expression is the minimum eigenvector at the maximizing value of $\mathbb E[ (x + G \omega) (x + G \omega)^T]$. 
\end{enumerate}

However, we do not operate with exact knowledge of $G$, etc. It turns out that even approximately solving this optimization problem with approximate values for $G, \Sigma, \mu$ suffices for our purposes. As long as the $\omega$ we obtain from our optimization (using the approximated values) results in a high value for the minimum eigenvalue of $\mathbb E[(x + G \omega) ( x + G \omega)^T] $. Let $\hat \omega$ be the maximizing value for the estimated optimization problem and let $\omega$ be the maximizing value for the original optimization problem. Let $Q$ be the maximizing matrix for the original problem and $\hat Q$ be the matrix resuling by replacing the true second moment, mean, $G$ the estimated ones. In formal terms, we need to show the following minimum eigenvalue of the following is large: $ \mathbb E [(x + G \hat \omega) (x + G \hat \omega)^T] $. 
We note that when $y^T \hat Q y$ within $\epsilon$ of $y^T Q y$ for all $y$ in the unit ball, the minimum eigenvalues may differ by at most $\epsilon$. 
\begin{align*}
    || y^T \hat Q y - y ^T Q y||^2 &= || y^T (\hat Q - Q) y||^2\\
    &\le \lambda_{max}^2 (\hat Q - Q)(y) || y ||^2\\
    & \le || \hat Q - Q||^2 
\end{align*}

And now we bound the norm of $|| \hat S - S ||^2$ assuming the following:
\begin{enumerate}
    \item $|| \hat S - S||^2 \le \epsilon $
    \item $|| \mu - \hat \mu ||^2 \le \frac{\lambda_{max}(G^T G) \epsilon}{d}$
    \item $|| \hat G - G ||^2 \le \frac \epsilon {d ||\mu||^2}$
    \item $|| \hat G - G ||^2 \le \frac{\epsilon} {d^2 || G ||^2}$
\end{enumerate}

We work out the bound below. 
\begin{align*}
    || \hat Q - Q ||^2 &= || S + 2 \mu {\omega^\star}^T G^T + G {\omega^\star} {\omega^\star}^T G^T - (\hat S + 2 \hat \mu \omega^T \hat G^T + \hat G  \omega^\star {\omega^\star}^T \hat G^T)||^2\\
    &\le || S - \hat S|| ^2 + 2||  \mu {\omega^\star}^T G^T -  \hat \mu {\omega^\star}^T \hat G^T|| ^2 + || \ldots|| ^2\\
    & \le \epsilon + 2||  \mu {\omega^\star}^T G^T  + {\hat \mu \omega^\star}^TG^T- {\hat \mu \omega^\star}^TG^T-  \hat \mu {\omega^\star}^T \hat G^T|| ^2 + || \ldots|| ^2\\
    &\le \epsilon + d|| \mu - \hat \mu||^2 ||  {\omega^\star}^T G ||^2 + || \hat G - G||^2 || \hat \mu \omega^T||^2 + \ldots\\
    &\le \epsilon + \epsilon + || \hat G - G||^2 || \hat \mu \omega^T  +\mu  \omega^T - \mu \omega^T ||^2 + \ldots\\
    &\le \epsilon + \epsilon + || \hat G - G||^2 (|| \hat \mu - \mu||^2 + || \mu {\omega^\star}^T||) + \ldots\\
    & \le \epsilon + \epsilon + || \hat G - G||^2 d || \mu||^2 + \ldots\\
    & \le 3 \epsilon + || \hat G  \omega^\star {\omega^\star}^T \hat G^T -  G  \omega^\star {\omega^\star}^T G^T ||^2\\
    &\le 3 \epsilon + || \hat G  \omega^\star {\omega^\star}^T \hat G^T - \hat G \omega^\star {\omega^\star}^T G + \hat G \omega^\star {\omega^\star}^T G -  G  \omega^\star {\omega^\star}^T G^T ||^2\\
    &\le 3 \epsilon + || (\hat G - G)  \omega^\star {\omega^\star}^T \hat G^T ||^2 + || (\hat G - G)  \omega^\star {\omega^\star}^T G^T ||^2\\
    & \le 3 \epsilon + || (\hat G - G)  \omega^\star {\omega^\star}^T \hat G^T - (\hat G - G)  \omega^\star {\omega^\star}^T G^T + (\hat G - G)  \omega^\star {\omega^\star}^T  G^T ||^2 + d^2|| \hat G - G||^2 ||G ||^2\\
    & \le 4 \epsilon  + ||(\hat G - G)  \omega^\star {\omega^\star}^T  (\hat G - G) ||^2 + || (\hat G - G)  \omega^\star {\omega^\star}^T G^T ||^2\\
    & \le 5 \epsilon + d^2 || \hat G - G||^4 \\
    & \le 6 \epsilon 
\end{align*}

This means if we find an $\epsilon-$approximate solution to the system with the estimated values, get a $\kappa_{min}$ within $2\epsilon$ of the optimal. 

\subsection{Recovering the causal estimator}
We can now describe the algorithm for recovering an estimate of the causal estimator. 

We start by estimating the parameters of the distribution of $x$. We set $\omega = 0$ and collect $O(\max (\frac{d \lambda_{max}(G^TG)}{ \kappa_{min}}), \frac{d^2 || S||^2}{\kappa_{min}}) $ samples. This suffices to recover $S$ within $O(\kappa_{min})$ squared frobenius norm and $\mu$ within $O(\frac{\kappa_{min} \lambda_{max}(G^T G)}{d})$ squared $\ell_2$ norm.  

We then run the procedure to estimate $G$, recovering it to squared $\ell_2$ norm error at most $O(\min(\frac{\kappa_{min}||\mu||^2}{d},\frac{\epsilon || G||^2}{d^2}))$. 

We then compute the most informative $\omega$ using the convex optimization described above. We solve it using a derivative free optimization technique such as the ellipsoid method. This $\omega$ is guaranteed to give us an expected moment matrix with minimum eigenvalue at least $\kappa_{min}/3$. 

We then simply collect $O( \frac{d}{\epsilon \kappa_{min}})$ samples, run OLS and use the recovered $\omega$ as our estimate of the causal classifier.
